# Supplementary material for: Quantitative Analysis of Image Classification Techniques for Memory-Constrained Devices
Source: arXiv:2005.04968 source file (2020-11-15)
Supplement: Supplementary file 1 [file appendix.tex]

%%%%%%%%%%%%
% Appendix %
%%%%%%%%%%%%

\appendix
\section{Hyperparameters}
\label{appendix:hyperparameters}

To encourage reproducibility of our experiments, we provide in this appendix all hyperparameter settings for the various experiments in section \ref{sec:experiments}, broken down for each model described in \ref{sec:background}.

\subsection{Direct Convolution}

\subsection{ProtoNN}

\subsection{Bonsai}

\subsection{FastGRNN}
